# Supplementary material for: LLM4SR: A Survey on Large Language Models for Scientific Research
Source: arXiv:2501.04306 source file (2025-01-08)
Supplement: Supplementary file 1 [file 7_appendix.tex]

\appendix
% \newpage

% \input{Tables/discovery_methods}

% \input{Tables/discovery_benchmarks}

% \input{Tables/3_benchmarks}

% \input{Tables/paper_writing_eval}

% \input{Tables/5_dataset_evalmetrics}

% \input{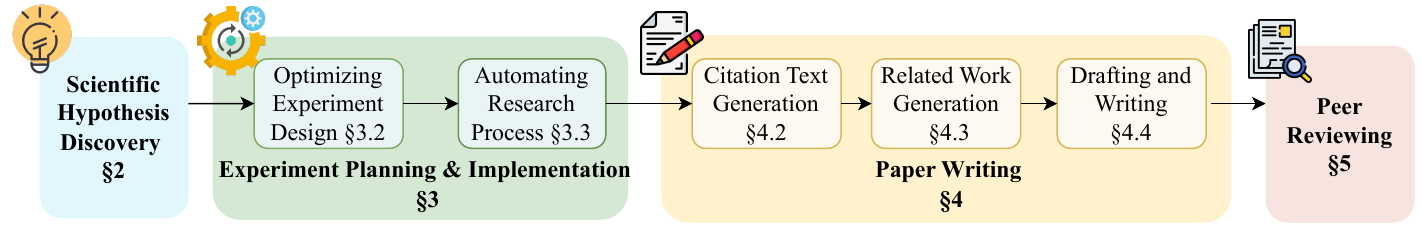}
% \input{Figures/category_tree}

% \input{Figures/schematic_overview}

\section{Appendix}

\subsection{Future Works}
\label{appendix:future_work}
\subsubsection{Scientific Hypotheses Discovery}
\label{appendix:scientific_hypotheses}

The first line of future work is to enhance the ability for automated experiment conduction~(or automated hypotheses validation), since it is the only reliable way to test the validness of a hypothesis.
It might appear differently in different disciplines. 
In computer science, the bottleneck might be the coding ability, especially the ability to program a large system.
In chemistry or biology, the bottleneck might lie in the robotics methods to conduct experiments~\citep{boiko2023autonomous}.

The second line of future work is to enhance the LLM's ability on hypotheses generation. 
Currently it is still not clear how to increase this ability.
The aspects might include training data collection method, and training strategy.

\subsubsection{Experiment Planning and Implementation}
\label{appendix:experiment_planning}
To overcome these challenges, techniques like data augmentation can improve the robustness and generalizability of LLMs. Advancing methods for model transparency and creating user-friendly interfaces will help researchers better understand LLM outputs. Establishing clear ethical guidelines and strategies to mitigate biases are essential for responsible use. Finally, developing interoperability standards and customizable solutions will facilitate integration with existing research tools.

\subsubsection{Scientific Paper Writing}
\label{appendix:paper_writing}

% \paragraph{Future Directions} 
To overcome these challenges, future advancements should focus on improving retrieval systems and enhancing models' capacity to synthesize information from diverse, long-context sources~\citep{li2022automatic, li2024related}. This includes developing better citation validation mechanisms, improving multi-document synthesis, and introducing real-time literature discovery to keep generated content up to date.
Additionally, incorporating domain-specific fine-tuning and reasoning-aware models will help generate more accurate, contextually relevant scientific text~\citep{moosavi2021scigen}. Fine-grained control over the writing process, such as adjusting tone and style, will also be crucial for making LLMs more adaptable to different academic needs~\citep{chen-etal-2021-scixgen-scientific, gao-etal-2023-enabling}.

\subsubsection{Peer Reviewing}
\label{appendix:peer_reviewing}

% From a data perspective, limited domain-specific datasets restrict the generalizability of LLM-based reviews, hindering their application across diverse fields \cite{zeng_2024_scientificopinionsummarizationpaper, Kang_2018_PeerReadDataset}. 
% \paragraph{Future Directions}
Future research must address challenges of integrating LLMs into peer review. Enhancing LLMs' ability to deliver critical evaluations is a key priority, including improving reasoning over long texts, identifying technical weaknesses, and developing methods for structured, coherent generation \cite{Zhou_2024_LLMReliableReviewer, Liu_2023_ReviewerGPT, Chenhui_2022_MReDDataset}. Incorporating domain-specific knowledge and optimizing prompts can further enhance accuracy as well. Human-in-the-loop systems present a promising approach, combining LLM efficiency with human judgment to mitigate biases and uphold ethical standards \cite{Drori_2024_HumanInTheLoopAIReviewing, Biswas_2023_ChatGPTJournalReviews}. Developing clear guidelines, governance strategies, and training for responsible LLM use will be crucial in ensuring transparency, accountability, and the integrity of the LLM-based peer review process.
